# Supplementary material for: Command of Collective Dynamics by Topological Defects in Spherical Crystals
Source: arXiv:1906.03977 source file (2019-06-10)
Supplement: Supplementary file 1 [file Supplemental_Material.pdf]

# Supplemental Material

Zhenwei Yao*

*School of Physics and Astronomy, and Institute of Natural Sciences,*

*Shanghai Jiao Tong University, Shanghai 200240, China*

## I. EQUATIONS OF MOTION: DERIVATION AND NUMERICAL INTEGRATION

Consider a collection of interacting point particles confined on the sphere of radius $R$. The particles labeled $i$ and $j$ interact by the potential $V(r_{ij})$, where $r_{ij}$ is the distance between the particles $i$ and $j$. $r_{ij}^2/2R^2 = 1-\cos\theta_i\cos\theta_j - \sin\theta_i\sin\theta_j\cos(\phi_i-\phi_j)$, where $\theta_i$ and $\phi_i$ are the polar and azimuthal angles of the particle $i$. The Lagrangian of the $N$-particle system is [1]

$$L = \sum_{i=1}^{N}\frac{1}{2}mR^2(\dot{\theta}_i^2+\sin^2\theta_i\dot{\phi}_i^2) - \sum_{i\neq j}V(r_{ij}), \tag{1}$$

where $m$ is the mass of the particle. From Eq.(1), we derive for the equations of motion in spherical coordinates

$$\begin{aligned} mR^2\ddot{\theta}_i &= mR^2\dot{\phi}_i^2\sin\theta_i\cos\theta_i - \sum_{j\neq i}\frac{\partial V(r_{ij})}{\partial\theta_i}, \\ mR^2\frac{d}{dt}\left(\sin^2\theta_i\dot{\phi}_i\right) &= -\sum_{j\neq i}\frac{\partial V(r_{ij})}{\partial\phi_i}. \end{aligned} \tag{2}$$

Eqs.(6) are invariant under the variable transformation of $\theta\to\theta+m\pi$ and $\phi\to\phi+2n\pi$, where $m$ and $n$ are integers. We note that, for a collection of free particles with $V(r)=0$, Eqs.(6) become the geodesic equations on the sphere.

We numerically integrate Eqs.(6) for the particle trajectories with various given initial conditions. By making use of $\dot{f}(t) = (f(t+h)-f(t))/h$ and $\ddot{f}(t) = (f(t+2h)+f(t)-$

*Electronic address: zyao@sjtu.edu.cn

$2f(t+h))/h^2$, we obtain the corresponding difference equations of Eqs.(6):

$$\begin{aligned}\theta(t+2h) &= 2\theta(t+h) - \theta(t) + \sin\theta(t)\cos\theta(t) \times (\phi(t+h) - \phi(t))^2 + h^2 F_\theta(t), \\ \phi(t+2h) &= \phi(t+h) + \frac{1}{\sin^2\theta(t+h)}[h^2 \sin\theta(t) F_\phi(t) + \sin^2\theta(t)(\phi(t+h) - \phi(t))], \quad (3)\end{aligned}$$

where we have ignored the subscripts in $\theta_i$ and $\phi_i$, and set $R = 1$ for clarity. We adjust the time step $h$ to be sufficiently fine to ensure that the total energy is well conserved. Typically, $h = 10^{-6}$. For the case of $\Gamma = 10\%$ and $(p, q) = (10, 0)$, over a million time steps, the total energy $E = 484996 \pm 1$. The highly conserved energy reflects the reliability of our numerical solution. In Eqs.(3), the relevant term associated with $F_\phi$ diverges at the north and south poles ($\theta = 0$ and $\pi$). To avoid divergence, we remove the small caps at the two poles of the sphere. In our numerical scheme, we set the criterion that once a particle moves into the region of $\theta < \theta_c$ or $\theta > \pi - \theta_c$, its position is reset to $\theta = \theta_c$ or $\theta = \pi - \theta_c$, respectively. We specify a vanishingly small value to $\theta_c$ such that almost no particle enters this forbidden zone in the entire simulation process.

Regarding the force terms in Eqs.(3), the force on a particle concerned at time $t$ is $\vec{F}(t) = F_\theta(t)\hat{e}_\theta + F_\phi(t)\hat{e}_\phi$, where $\hat{e}_\theta$ and $\hat{e}_\phi$ are the normal basis vectors at the position of the particle concerned. Using $\nabla f = \frac{1}{R}\frac{\partial f}{\partial \theta}\hat{e}_\theta + \frac{1}{R\sin\theta}\frac{\partial f}{\partial \phi}\hat{e}_\phi$, we have $F_{\theta_i} = -\frac{1}{R}\sum_{j\neq i}\frac{\partial V(r_{ij})}{\partial \theta_i}$ and $F_{\phi_i} = -\frac{1}{R\sin\theta_i}\sum_{j\neq i}\frac{\partial V(r_{ij})}{\partial \phi_i}$. Here, we record the force on particle $i$ by particle $j$ as:

$$\begin{aligned}\vec{F}_{ij} &= -\nabla_i V(r_{ij}) \\ &= \alpha\beta r_{ij}^{-\alpha-2}[(\sin\theta_i\cos\theta_j - \cos\theta_i\sin\theta_j \times \cos(\phi_i - \phi_j))\hat{e}_{\theta_i} \\ &\qquad + \sin\theta_j \sin(\phi_i - \phi_j)\hat{e}_{\phi_i}]. \quad (4)\end{aligned}$$

The initial conditions for Eqs.(3) are specified by the displacement of the particles with respect to their balance positions. $\delta\vec{x} = (R\delta\theta, R\sin\theta\delta\phi) = \Gamma a(\cos\alpha, \sin\alpha)$, where the basis vectors are $\{\hat{e}_\theta, \hat{e}_\phi\}$. $\Gamma$ represents a fraction of the lattice spacing. $\delta\vec{x}$ is a tangent vector at the position of the particle concerned. The amount of particle displacement in terms of $\delta\theta$ and $\delta\phi$ is: $\delta\theta = \Gamma a\cos\alpha$, and $\delta\phi = \Gamma a\sin\alpha/\sin\theta$. $\Gamma$ and $\alpha$ represent the magnitude and direction of the particle displacement. With the initial conditions of $\theta(t=0) = \theta_0$, $\phi(t=0) = \phi_0$, $\dot{\theta}(t=0) = 0$ and $\dot{\phi}(t=0) = 0$, we have $\theta(t=h) = \theta(t=0)$ and $\phi(t=h) = \phi(t=0)$. With these initial inputs, we can compute for the particle trajectory $\{\theta(t), \phi(t)\}$ from Eqs.(3). To avoid abrupt change in the spherical coordinates, we make use

of the invariance of the equations of motion under the above-mentioned translation of the spherical coordinates, and lift the limit for the allowed values of $\theta$ and $\phi$.

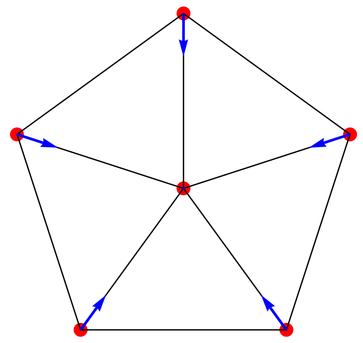

FIG. 1: The radial mode derived in the normal mode analysis of the elementary pentagonal configuration. The red dots represent identical particles of mass $m$, which are connected by identical springs of stiffness $k_0$. In such a mode, the central particle has zero velocity. This is exactly the mode selected by the system to fabricate the breathing mode. The eigenfrequency of the radial mode is $\omega = \frac{1}{2}\left(7-\sqrt{5}\right)\sqrt{\frac{k_0}{m}}$.

## II. NORMAL MODE ANALYSIS FOR ELEMENTARY PENTAGONAL CONFIGURATIONS

To further our understanding about the breathing mode around the five-fold disclinations, we perform normal mode analysis of the elementary pentagonal configuration. It consists of six identical point particles of mass $m$: a central particle surrounded by five neighboring particles. In the regime of small perturbation, the interaction between neighboring particles can be well approximated by harmonic potential. The central particle is connected by five neighboring particles with identical springs of stiffness $k_0$. The surrounding particles are also connected by identical springs of stiffness $k_1$. Such an elementary pentagonal mass-spring system is named $P_6$ configuration. Since the sphere as a smooth Riemannian manifold is locally flat and the $P_6$ configuration occupies a very small area over the sphere, we assume that the vibrations of the particles are confined on the plane in our derivation.

In the equilibrium configuration, the distance between the central particle and any neighboring particle is $a$, and the distance between any neighboring particles is $b$. $b = 2a\sin(\alpha/2)$. $\alpha = 2\pi/5$. The eigenmodes of vibration of the $P_6$ configuration can be derived by the follow-

ing standard normal mode analysis. Considering a collection of $N$ identical point particles whose positions are deviated from the equilibrium configuration $\{q_{0i}\}$ $(i = 1, 2, 3...N)$. The Lagrangian of the system is

$$L = \frac{1}{2} T_{ij} \dot{\eta}_i \dot{\eta}_j - \frac{1}{2} V_{ij} \eta_i \eta_j. \tag{5}$$

$\eta_i = q_i - q_{i0}$, which is the deviation of the generalized coordinate from its equilibrium value. $V_{ij} = (\frac{\partial^2 V}{\partial q_i \partial q_j})_0$, which is evaluated at the equilibrium configuration. $T_{ij} = m\delta_{ij}$, where $m$ is the particle mass. The Lagrangian leads to the following $n$ equations of motion:

$$T_{ij} \ddot{\eta}_j + V_{ij} \eta_j = 0. \tag{6}$$

The general solution of the equations of motion can be written as a summation over an index $k$:

$$\eta_i = C_k a_{ik} \exp(-i\omega_k t). \tag{7}$$

By inserting Eq.(7) into Eq.(6), we obtain the equations of motion for the $k$-mode:

$$(V_{ij} - T_{ij}\omega_k^2) a_{jk} = 0. \tag{8}$$

Note that no summation over $k$ is applied in the above equation. We solve for the eigenvalue $\omega_k$ by requiring the determinant of $(V_{ij} - T_{ij}\omega_k^2)$ to be zero, and calculate the corresponding eigenvector based on Eq.(8).

Now, we apply the above formalism to the $P_6$ configurations. We first investigate the case of $k_1 = k_0$. All the derived eigenfrequencies are listed below (measured in the unit of $\sqrt{k_0/m}$):

$$\begin{aligned} \omega_{1,2,3} &= 0, & \omega_{4,5} &= \frac{1}{2}\left(5 - \sqrt{5}\right), \\ \omega_{6,7} &= \frac{3}{4}\left(3 + \sqrt{5}\right), & \omega_{8} &= \frac{1}{2}\left(7 - \sqrt{5}\right), \\ \omega_{9,10} &= \frac{1}{4}\left(7 - \sqrt{29 - 8\sqrt{5}}\right), & \omega_{11,12} &= \frac{1}{4}\left(7 + \sqrt{29 - 8\sqrt{5}}\right). \end{aligned} \tag{9}$$

The subscripts represent the twelve eigenvectors. Both the total momentum and angular moment of all the normal modes are zero. The first three eigenmodes with zero-frequency correspond to the two translational and one rotational degrees of freedom. Notably, the $P_6$ configuration does not support any other zero-energy modes called floppy modes which

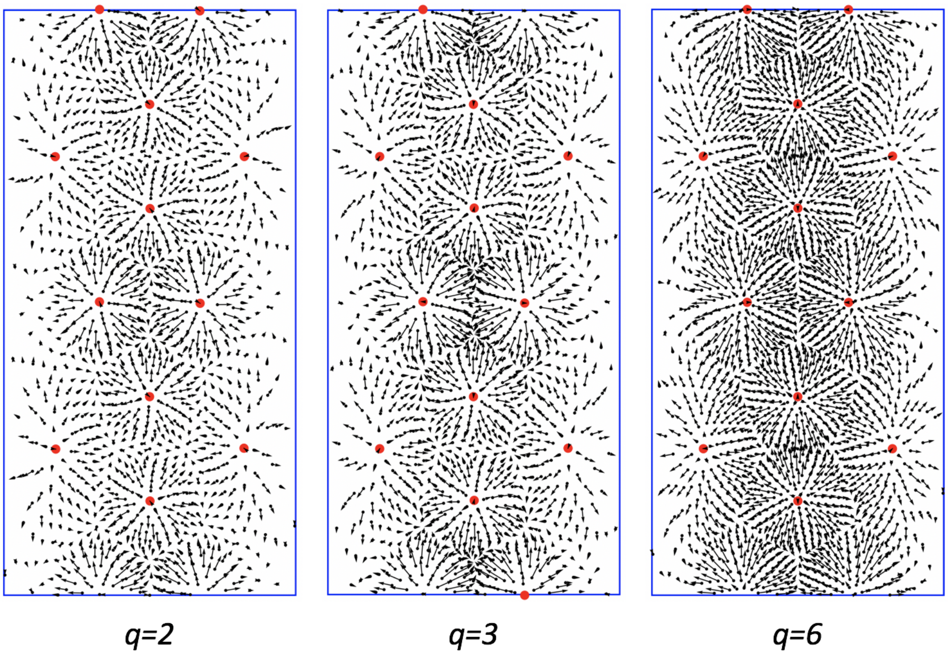


FIG. 2: Velocity fields in spherical crystals with non-zero $q$-values. They have the identical singularity structure as that of the spherical crystal with $q = 0$. The red dots are the pre-existent five-fold disclinations. $p = 10$. $\Gamma = 0.01$.

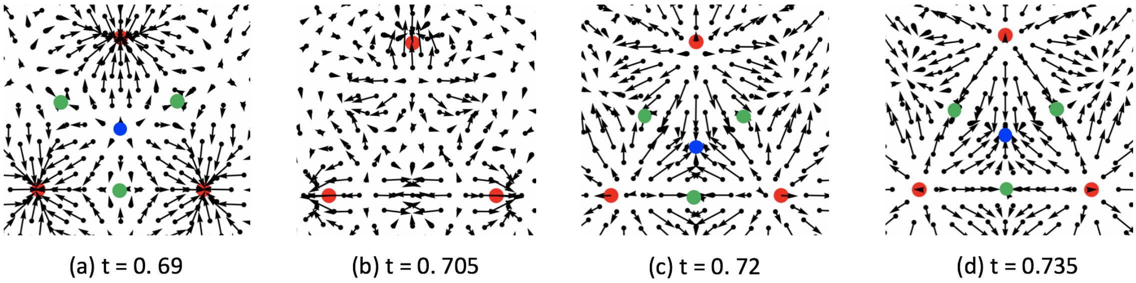


FIG. 3: Typical instantaneous velocity fields. The velocity field of an elementary triangular region over the spherical crystal is shown for visual convenience. The velocity vectors near the disclinations (indicated by red dots) are pointing inward (a) and outward (d). The three types of singularities (see Fig. 1 in the main text) are indicated with different colors. $\Gamma = 1\%$. $(p, q) = (10, 0)$.

originate from the insufficient number of constraints to match the total number of degrees of freedom [2, 3].

Among all the twelve normal modes in the $P_6$ configuration, only the $\omega_8$ mode (radial mode), whose eigenvector is shown in Fig. 1, preserves the $C_5$ symmetry of the $P_6$ configu-

ration. To check if the $P_6$ configuration also supports the radial mode with the variation of $k_1/k_0$, we perform calculations for the cases of $k_1/k_0 = 1/2 < 1$ and $k_1/k_0 = 3/2 > 1$, and find radial modes in both kinds of systems, but at different eigenfrequencies. Specifically, for the case of $k_1/k_0 = 1/2$,

$$\omega_{\mathrm{radial}} = \frac{1}{4}\left(9-\sqrt{5}\right)\sqrt{\frac{k_0}{m}}, \tag{10}$$

and for the case of $k_1/k_0 = 3/2$,

$$\omega_{\mathrm{radial}} = \frac{1}{4}\left(19-3\sqrt{5}\right)\sqrt{\frac{k_0}{m}}. \tag{11}$$

To conclude, the radial mode derived in the normal mode analysis for elementary pentagonal configurations is exactly the mode selected in the collective dynamics of the spherical crystal to fabricate the breathing mode.

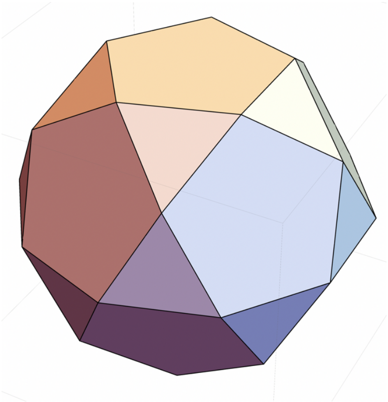

FIG. 4: Plot of an icosidodecahedron. The 30 singularities indicated by green dots in the velocity field of the spherical crystal (see Fig.2 in the main text) constitute a dodecahedron.

## III. VELOCITY FIELD CONFIGURATIONS

### A. $q \neq 0$ cases

In Fig. 2, we present the typical velocity fields in spherical crystals with $q = 2$, 3, and 6, which reflect distinct symmetries of the spherical crystal. $p = 10$. The red dots are the pre-existent five-fold disclinations. The vector field converges towards the centers of the triangles spanned by three neighboring red dots; these sites are labeled by blue dots

in Fig.2 in the main text. Symmetry consideration shows that the midpoints of the edges connected by neighboring red dots are the saddle points in the vector field, corresponding to the green dots in Fig.2 in the main text. Therefore, the velocity fields of spherical crystals with nonzero $q$ have the identical singularity structure as that of $q = 0$.

### B. Evolution of velocity field

In Fig. 3, we present the typical instantaneous velocity fields over an elementary triangular region in the spherical crystal. The velocity vectors near the disclinations (indicated by red dots) are pointing inward in Fig. 3(a) and outward in Fig. 3(d). We observe the slight movement of the singularities in the velocity field, which are indicated with different colors. Due to the discreteness of the system, the singularity structure in Fig. 3(b) is barely distinguishable; slight displacement of singularities is expected in the continuum limit.

### C. Icosidodecahedron

In Fig. 2 in the main text, we have shown that the 20 blue dots in the velocity field constitute an inscribed dodecahedron. In Fig. 4, we present the shape of an icosidodecahedron. It has 30 identical vertices, 60 identical edges, 20 triangular faces and 12 pentagonal faces. Two triangles and two pentagons meet at each vertex. Each edge separates a triangle from a pentagon.

## IV. DRIFT OF DISCLINATIONS IN MELTING SPHERICAL CRYSTALS

In the melting of the spherical crystal at sufficiently large $\Gamma$, we have shown that the relative positions of the pre-existent disclinations are subject to large deviation from their original balance positions due to the softening of the crystal lattice (see Fig.4 in the main text). In Fig. 5, we present the detailed information about the time evolution of the angular separation $\alpha_{ij}$ between two disclinations labeled $i$ (any of the twelve pre-existent disclinations) and $j$. From the straight lines in Fig. 5(a), we see that for small $\Gamma$, the disclinations are well anchored in their original positions. When melting occurs at larger $\Gamma$, the disclinations

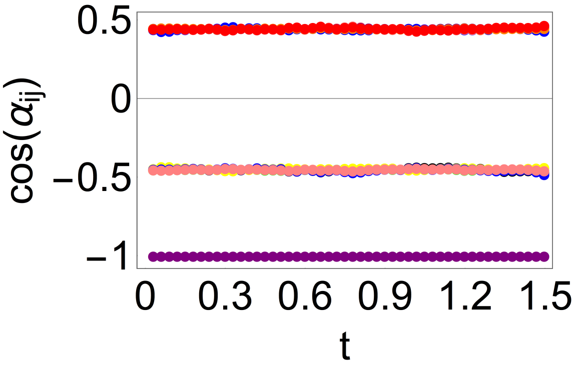


(a)

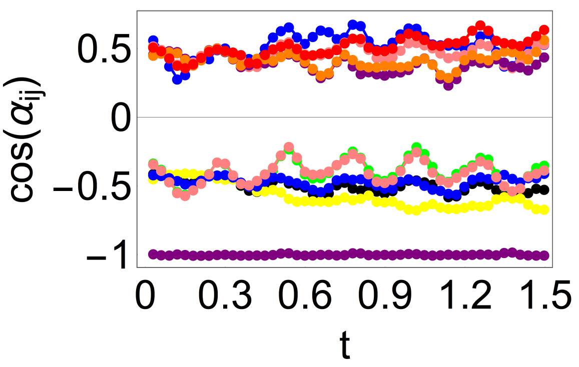


(b)

FIG. 5: Drift of disclinations with the increase of Γ. $\alpha_{ij}$ is the angle between a disclination labeled $i$ and one of the other eleven disclinations. $\Gamma = 1\%$ (a) and 60% (b). $(p, q) = (10, 0)$.

start to drift away from the balance positions, as shown in Fig. 5(b).

---


[1] H. Goldstein, *Classical mechanics* (Pearson Education India, 2011).

[2] J. C. Maxwell, Philos. Mag. **27**, 294 (1864).

[3] V. Vitelli, PNAS **109**, 12266 (2012).
